# Supplementary material for: Real-Time Verification for Distributed Cyber-Physical Systems
Source: arXiv:1909.09087 source file (2019-09-19)
Supplement: Supplementary file 1 [file appendix.tex]

\appendix

\section{Safety properties of ACAS Xu networks}
We present a list of properties that are checked to be satisfied or unsatisfied by ACAS Xu benchmarks.  \cite{katz2017reluplex}
\begin{itemize}
	\item \textbf{Property $\phi_1$.}
	\begin{itemize}
		\item If the intruder is distant and is significantly slower than the ownship, the score of a \textit{COC} advisory will always be below a certain fixed threshold.
		\item The desired output property is that the score for COC is at most 1500.
		\item It has 3 input constraints: $\rho$ $\geq$ 55947.691, $v_{own}$ $\geq$ 1145, $v_{int}$ $\leq$ 60.
	\end{itemize}
	\item \textbf{Property $\phi_2$.}
	\begin{itemize}
		\item If the intruder is distant and is significantly slower than the ownship, the score of a \textit{COC} advisory will never be maximal.
		\item The desired output property is that the score for COC is not the maximal score.
		\item It has 3 input constraints: $\rho$ $\geq$ 55947.691, $v_{own}$ $\geq$ 1145, $v_{int}$ $\leq$ 60.
	\end{itemize}
	\item \textbf{Property $\phi_3$.}
	\begin{itemize}
		\item If the intruder is directly ahead and is moving towards the ownship, the score for \textit{COC} will not be minimal.
		\item The desired output property is that the score for COC is not the minimal score.
		\item It has 5 input constraints: 1500 $\leq$ $\rho$ $\leq$ 1800, $\theta$ $\leq$ $|0.06|$,  $\psi$ $\geq$ 3.10, $v_{own}$ $\geq$ 980, $v_{int}$ $\geq$ 960.
	\end{itemize}
	\item \textbf{Property $\phi_4$.}
	\begin{itemize}
		\item If the intruder is directly ahead and is moving away from the ownship but at a lower speed than that of the ownship, the score for \textit{COC} will not be minimal.
		\item The desired output property is that the score for COC is not the minimal score.
		\item It has 5 input constraints: 1500 $\leq$ $\rho$ $\leq$ 1800, $\theta$ $\leq$ $|0.06|$,  $\psi$ = 0, $v_{own}$ $\geq$ 1000, 700 $\leq$ $v_{int}$ $\leq$ 800.
	\end{itemize}
	\item \textbf{Property $\phi_5$.}
	\begin{itemize}
		\item If the intruder is near and approaching from the left, the network advises \textit{strong right}.
		\item The desired output property is that the score for strong right is the minimal score.
		\item It has 5 input constraints: 250 $\leq$ $\rho$ $\leq$ 400, 0.2 $\leq$ $\theta$ $\leq$ 0.04, -3.141592 $\leq$ $\psi$ $\leq$ -3.141592+0.005, 100 $\leq$ $v_{own}$ $\leq$ 400, 0 $\leq$ $v_{int}$ $\leq$ 400.
	\end{itemize}
	\item \textbf{Property $\phi_6$.}
	\begin{itemize}
		\item If the intruder is sufficiently far away, the network advises \textit{COC}.
		\item The desired output property is that the score for COC is the minimal score.
		\item It has 5 input constraints: 12000 $\leq$ $\rho$ $\leq$ 62000, (0.7 $\leq$ $\theta$ $\leq$ 3.141592 $\vee$ (-3.141592 $\leq$ $\theta$ $\leq$ -0.7), -3.141592 $\leq$ $\psi$ $\leq$ -3.141592+0.005, 100 $\leq$ $v_{own}$ $\leq$ 1200, 0 $\leq$ $v_{int}$ $\leq$ 1200.
	\end{itemize}
	\item \textbf{Property $\phi_7$.}
	\begin{itemize}
		\item If vertical separation is large, the network will never advise a strong turn.
		\item The desired output property is that the scores for strong right and strong left are never the minimal scores.
		\item It has 5 input constraints: 0 $\leq$ $\rho$ $\leq$ 60760,  -3.141592 $\leq$ $\theta$ $\leq$  3.141592, -3.141592 $\leq$ $\psi$ $\leq$ 3.141592, 100 $\leq$ $v_{own}$ $\leq$ 1200, 0 $\leq$ $v_{int}$ $\leq$ 1200.
	\end{itemize}
	\item \textbf{Property $\phi_8$.}
	\begin{itemize}
		\item For a large vertical separation and a previous \textit{weak left} advisory, the network will either output \textit{COC} or continue advising \textit{weak left}.
		\item The desired output property is that the score for weak left is minimal or the score for COC is minimal.
		\item It has 5 input constraints: 0 $\leq$ $\rho$ $\leq$ 60760,  -3.141592 $\leq$ $\theta$ $\leq$ -0.75 x 3.141592, -0.1 $\leq$ $\psi$ $\leq$ 0.1, 600 $\leq$ $v_{own}$ $\leq$ 1200, 600 $\leq$ $v_{int}$ $\leq$ 1200.
	\end{itemize}
	\item \textbf{Property $\phi_9$.}
	\begin{itemize}
		\item Even if the previous advisory was \textit{weak right}, the presence of a nearby intruder will cause the network to output a \textit{strong left} advisory instead.
		\item The desired output property is that the score for strong left is minimal.
		\item It has 5 input constraints: 2000 $\leq$ $\rho$ $\leq$ 7000,  -0.4 $\leq$ $\theta$ $\leq$ -0.14, -3.141592 $\leq$ $\psi$ $\leq$ -3.141592+0.01, 100 $\leq$ $v_{own}$ $\leq$ 150, 0 $\leq$ $v_{int}$ $\leq$ 150.
	\end{itemize}
	\item \textbf{Property $\phi_{10}$.}
	\begin{itemize}
		\item For a far away intruder, the network advises \textit{COC}.
		\item The desired output property is that the score for COC is minimal.
		\item It has 5 input constraints: 36000 $\leq$ $\rho$ $\leq$ 60760,  0.7 $\leq$ $\theta$ $\leq$ 3.141592, -3.141592 $\leq$ $\psi$ $\leq$ -3.141592+0.01, 900 $\leq$ $v_{own}$ $\leq$ 1200, 600 $\leq$ $v_{int}$ $\leq$ 1200.
	\end{itemize}
\end{itemize}
